# Supplementary material for: Homophily-enhanced Structure Learning for Graph Clustering
Source: arXiv:2308.05309 source file (2023-10-30)
Supplement: Supplementary file 1 [file appendix.tex]

\section{Algorithm}
\label{sec:alg}

Here we present the complete training algorithm as Algorithm \ref{algorithm}.

\begin{algorithm}
  \caption{\titlename}
  \label{algorithm}
  \begin{algorithmic}[1]
    \Require Original graph $\mathcal{G}(\mathcal{V},\mathbf{X},\mathcal{E}, \mathbf{A})$, number of clusters $K$, embedding dimension $d$, maximum number of structure learning epochs $\text{max\_epoch}$
    \Ensure Cluster assignments $\mathbf{C}$
        \State Train GNN using original structure $\mathbf{A}$ by Equation \eqref{eqn:reg} to obtain node embedding $\mathbf{Z}$;
        \State Initialize the cluster centers $\mu$ based on $\mathbf{Z}$ using K-means;
        \State Jointly train GNN and clustering by Equation \eqref{eqn:reg} and \eqref{eqn:cls};
        \For {epoch=0 \textbf{to} $\text{max\_epoch}$ }
            \State Update cluster soft assignments $\mathbf{Q}$ by Equation \eqref{eqn:Q};
            \State Update structure $(\widebar{\mathcal{E}},\mathbf{\widebar{A}})$ with cluster soft assignments $\mathbf{Q}$ by Equation \eqref{eqn:Erc} and \eqref{eqn:Erm};
            \State Jointly train GNN and clustering with $(\widebar{\mathcal{E}},\mathbf{\widebar{A}})$ by Equation \eqref{eqn:reg} and \eqref{eqn:cls};
        \EndFor
  \State Get the cluster hard assignments by $\mathbf{C}=\argmax\mathbf{Q}$.
  \end{algorithmic}
\end{algorithm}

\section{Reproducibility}
Here are more details about the experiments to help with reproducibility.

\begin{table}[]
  \caption{Hardware and Software Configurations}
  \resizebox{1.0\columnwidth}{!}{
    \begin{tabular}{ll}
    \toprule[0.8pt]
    \multicolumn{2}{c}{\textbf{Hardware}}                                                     \\ \hline
    \multicolumn{1}{l|}{\textbf{Operating System}} & Ubuntu 18.04.6 LTS                        \\ 
    \multicolumn{1}{l|}{\textbf{GPU}}              & NVIDIA GeForce RTX 3090                   \\ 
    \multicolumn{1}{l|}{\textbf{CPU}}              & Intel(R) Xeon(R) CPU E5-2680 v4 @ 2.40GHz \\\hline 
    \multicolumn{2}{c}{\textbf{Software}}                                                     \\ \hline
    \multicolumn{1}{l|}{\textbf{Python}}           & 3.6.2                                     \\ 
    \multicolumn{1}{l|}{\textbf{torch}}            & 1.9.1+cu111                               \\ 
    \multicolumn{1}{l|}{\textbf{scikit-learn}}     & 0.24.2                                    \\ 
    \multicolumn{1}{l|}{\textbf{scipy}}            & 1.5.4                                     \\ 
    \bottomrule[0.8pt]
    \end{tabular}
  }
  \label{tab:hardware}
\end{table}

\subsection{Hardware and Software Configurations}
All experiments are conducted on a server under the same environment in Table \ref{tab:hardware}.
% Hardware:
% \begin{itemize}
%   \item Operating System: Ubuntu 18.04.6 LTS
%   \item GPU: NVIDIA GeForce RTX 3090
%   \item CPU: Intel(R) Xeon(R) CPU E5-2680 v4 @ 2.40GHz
% \end{itemize}
% Software:
% \begin{itemize}
%   \item Python 3.6.2
%   \item torch 1.9.1+cu111
%   \item scikit-learn 0.24.2
%   \item scipy 1.5.4
% \end{itemize}

\subsection{Hyperparamenter Settings}

We report our hyperparameter settings in Table \ref{tab:hyper-param}.

\begin{table}[]
    \caption{Hyperparamenter Settings. Ep. is short for GSL epochs.  $\gamma$ is the percentage of nodes with the highest cluster assignment probability for edge recovery, while $\xi$ and $\eta$ are the intra-cluster edge recovery ratio and inter-cluster edge removal ratio respectively. $l$ is the number of feature propagation times, and $t$ is the number of linear transformation layers. lr is short for learning rate, and Dim. is an abbreviation for the dimension of output embedding.}
    \resizebox{.48\textwidth}{!}{
        \begin{tabular}{c|c|c|c|c|c|c|c}
            \toprule[0.8pt]
                     & \textbf{Flickr} & \textbf{Blog} & \textbf{Citeseer} & \textbf{ACM} & \textbf{Pubmed} & \textbf{Reddit} & \textbf{Cora} \\ \hline
            \textbf{Ep.}      & 10              & 10            & 5                 & 10           & 3               & 1               & 5             \\
            $\gamma$ & 0.5             & 1.0           & 0.3               & 0.3          & 0.5             & 0.01            & 1.0           \\
            $\xi$    & 0.5             & 0.5           & 0.5               & 0.5          & 0.5             & 0.005           & 0.5           \\
            $\eta$   & 0.005           & 0.005         & 0.005             & 0.005        & 0.005           & 0.02            & 0.01          \\
            $l$      & 1               & 1             & 3                 & 3            & 35              & 3               & 8             \\
            $t$      & 1               & 1             & 1                 & 1            & 1               & 1               & 1             \\
            lr       & 1e-3            & 1e-3          & 1e-3              & 1e-3         & 1e-3            & 2e-5            & 1e-3          \\
            \textbf{Dim.}     & 500             & 500           & 500               & 500          & 500             & 500             & 500           \\
            \bottomrule[0.8pt]
        \end{tabular}
    }
    \label{tab:hyper-param}
\end{table}

\begin{table}[]
    \caption{Hyperparamenter Settings of Experiments on Heterophilous Graphs. Notations are the same as Table \ref{tab:hyper-param}}
    \resizebox{.48\textwidth}{!}{
        \begin{tabular}{c|c|c|c|c|c|c}
            \toprule[0.8pt]
                    & \textbf{Wisconsin} & \textbf{Texas} & \textbf{Cornell} & \textbf{Actor} & \textbf{Chameleon} & \textbf{Squirrel} \\ \hline
            \textbf{Ep.}      & 15              & 5            & 15                 & 1           & 1               & 1                          \\
            $\gamma$ & 0.3             & 0.2           & 0.3               & 0.1          & 0.5             & 0.3                     \\
            $\xi$    & 0.5             & 0.5           & 0.5               & 0.5          & 0.5             & 0.5          \\
            $\eta$   & 0.1           & 0.01         & 0.1             & 0.05        & 0.005           & 0.05            \\
            $l$      & 0               & 0             & 0                 & 0            & 0              & 1              \\
            $t$      & 1               & 1             & 1                 & 1            & 1               & 1                  \\
            lr       & 1e-3            & 1e-3          & 1e-3              & 1e-3         & 1e-3            & 1e-3                \\
            \textbf{Dim.}     & 500             & 500           & 500               & 500          & 500             & 500                   \\
            \bottomrule[0.8pt]
        \end{tabular}
    }
    \label{tab:hyper-param-heter}
\end{table}

\section{Additional Experiments}

Here we present additional experiments for a better understanding of our model \model.

\subsection{Experiment Results on Six Heterophilous Graphs}
\label{app: heterophily}

Additional experimental results concerning six heterophilous graphs are provided in  Table \ref{tab:heterophily} for reference. The respective hyperparameter configurations are presented in Table \ref{tab:hyper-param-heter}.

\begin{table*}[t]
    \centering
    \small
    \caption{Result on Six Heterophily Graphs. The best results are in bold, and the second-best results are underlined.}
    \resizebox{1.6\columnwidth}{!}{
          \begin{tabular}{c|c|c|c|c|c|c|c}
            \toprule[0.8pt]                  
       \textbf{DataSet} & \textbf{Metric} & \textbf{Wisconsin} & \textbf{Texas} & \textbf{Cornell} & \textbf{Actor} & \textbf{Chameleon} & \textbf{Squirrel} \\ 
        ~ & \textit{Homophily} & \textit{0.21} & \textit{0.11} & \textit{0.3} & \textit{0.22} & \textit{0.23} & \textit{0.22} \\ 
        \midrule[0.8pt]
        DGI & ARI & 8.62±1.49 & 23.42±1.9 & 5.32±0.88 & \textbf{3.57±0.36} & 5.96±0.07 & 1.31±0.07 \\ 
        ~ & NMI & 9.92±3.6 & 18.47±1.38 & 6.73±1.27 & \underline{2.68±0.47} & 9.54±0.52 & 2.13±0.05 \\ 
        ~ & ACC & 45.42±1.44 & 56.65±0.63 & 40.26±2.07 & \textbf{29.46±0.6} & 29.48±0.4 & 25.66±0.2 \\ \hline
        SEComm & ARI & 2.95±1.4 & 0.47±0.91 & 2.68±0.89 & 0.29±0.11 & \underline{11.87±0.61} & 0.5±0.44 \\ 
        ~ & NMI & 3.99±2.46 & 1.06±2.07 & 4.79±2.33 & 0.37±0.22 & \underline{15.67±1.54} & 1.26±1.11 \\ 
        ~ & ACC & 30.15±2.01 & 27.69±1.76 & 30.78±3.56 & 22.95±0.57 & \underline{34.11±0.55} & 23.06±2.62 \\ \hline
        DFCN & ARI & NA & NA & NA & 0.22±0.16 & 7.26±0.29 & 0.06±0.04 \\ 
        ~ & NMI & NA & NA & NA & 0.24±0.23 & 12.11±0.22 & 0.31±0.18 \\ 
        ~ & ACC & NA & NA & NA & 22.92±0.73 & 31.97±0.09 & 21.79±0.2 \\ \hline
        DCRN & ARI & 2.84±0.95 & 17.71±0.90 & 10.79±1.13 & 0.41±0.12 & 3.20±0.34 & \underline{1.92±0.86} \\ 
        ~ & NMI & 2.93±0.63 & 12.77±0.59 & 11.43±0.60 & 0.37±0.09 & 9.88±0.58 & \textbf{4.30±0.84} \\ 
        ~ & ACC & 46.75±0.38 & 57.92±0.45 & 50.64±1.03 & 24.18±0.10 & 32.99±0.82 & \textbf{27.45±1.64} \\ \hline
        GCC & ARI & 4.98±0.00 & 15.10±0.00 & 3.82±0.87 & 0.11±0.05 & 5.73±0.00 & 0.31±0.00 \\ 
        ~ & NMI & 8.75±0.00 & 11.82±0.00 & 3.86±1.15 & 0.05±0.01 & 7.59±0.00 & 0.60±0.00 \\ 
        ~ & ACC & 47.81±0.00 & 54.10±0.00 & 35.70±2.29 & 25.57±0.05 & 32.59±0.00 & 23.16±0.04 \\ \hline
        SUBLIME & ARI & \textbf{35.85±4.87} & \textbf{38.18±5.88} & \textbf{33.66±2.44} & 0.07±0.13 & 3.17±0.25 & 0.3±0.06 \\ 
        ~ & NMI & \underline{34.1±0.55} & \underline{32.23±2.58} & \underline{29.63±2.56} & 0.2±0.15 & 6.97±0.35 & 0.57±0.15 \\
        ~ & ACC & \underline{63.61±5.98} & \textbf{64.12±4.45} & \underline{60.66±2.73} & 23.86±0.14 & 30.99±0.72 & 23.31±0.34 \\ \hline
        \textbf{HoLe} & ARI & \underline{32.38±3.91} & \underline{32.04±1.58} & \underline{32.88±6.44} & \underline{3.35±0.29} & \textbf{14.86±0.43} & \textbf{2.03±0.17} \\ 
        ~ & NMI & \textbf{35.37±2.60} & \textbf{32.81±1.07} & \textbf{38.45±3.38} & \textbf{3.89±0.07} & \textbf{17.84±0.17} & \underline{2.14±0.37} \\ 
        ~ & ACC & \textbf{63.88±1.88} & \underline{62.66±0.63} & \textbf{61.20±4.86} & \underline{28.35±0.31} & \textbf{36.81±0.11} & \underline{26.17±0.36} \\
            \bottomrule[0.8pt]
            \end{tabular}
    }
    \label{tab:heterophily}
\end{table*}

\subsection{Experimental Results of Purity}
\label{app: purity}

We hereby present supplementary experimental results of purity in Table \ref{tab:purity}.

\begin{table*}[t]
    \centering
    \small
    \caption{Purity Results. The best results are in bold, and the second-best results are underlined.}
    \resizebox{2\columnwidth}{!}{
          \begin{tabular}{c|c|c|c|c|c|c|c|c}
            \toprule[0.8pt]                  
        DataSet & Cora & Citeseer & Pubmed & ACM & Blog & Flickr & Reddit & ogb-products \\ 
        \midrule[0.8pt]
        DGI & 73.95±1.9 & 72.03±0.15 & 66.28±0.25 & \underline{90.69±0.08} & 37.36±5.54 & 15.08±0.06 & OOM & OOM \\ \hline
        MVGRL & 37.68±4.08 & 52.69±3.99 & 46.04±2.53 & 40.82±1.93 & 28.69±3.37 & 15.35±1.72 & OOM & OOM \\ \hline
        SENet & 70.95±0.41 & 67.77±1.63 & 67.19±1.01 & 82.07±0.55 & NA & NA & OOM & OOM \\ \hline
        AGC & 69.79±0.0 & 69.55±0.08 & 70.14±0.02 & 79.91±0.04 & 32.81±0.21 & 22.58±0.33 & OOM & OOM \\ \hline
        DAEGC & 63.04±2.69 & 67.09±0.74 & OOM & 84.91±8.56 & 27.6±0.78 & 20.67±2.6 & OOM & OOM \\ \hline
        SDCN & 52.25±2.52 & 51.38±2.87 & 59.71±1.11 & 86.08±3.8 & 20.68±1.05 & 17.69±3.72 & 31.3±3.69 & OOM \\ \hline
        AGCN & 51.21±4.83 & 55.33±2.71 & 62.77±5.14 & 65.11±1.15 & 34.12±6.51 & 13.03±1.87 & \underline{59.29±1.67} & OOM \\ \hline
        DFCN & 54.3±4.49 & 64.92±1.36 & 66.18±0.31 & 83.6±2.9 & 27.42±2.08 & 13.47±0.54 & OOM & OOM \\ \hline
        DCRN & 58.14±4.66 & 70.34±0.26 & 70.36±0.11 & 89.28±0.22 & 25.89±0.21 & 16.53±1.18 & OOM & OOM \\ \hline
        SEComm & 51.54±9.02 & 45.51±11.48 & 55.28±6.87 & 52.93±17.99 & 39.04±4.61 & 24.83±3.7 & OOM & OOM \\ \hline
        AGC-DRR & 36.84±0.81 & 28.82±1.29 & 40.19±0.12 & 73.96±7.38 & 35.07±3.96 & 13.71±2.27 & OOM & OOM \\ \hline
        GCC & 64.27±0.71 & \textbf{72.19±0.05} & \underline{70.82±0.00} & 42.61±0.00 & 50.90±0.00 & 17.10±4.29 & 57.58±2.53 & OOM \\ \hline
        SUBLIME & 45.77±13.48 & 53.53±1.18 & OOM & 84.01±1.44 & \underline{75.81±1.83} & \underline{64.44±0.5} & OOM & OOM \\ \hline
        AGE & \underline{73.99±0.21} & 70.23±0.19 & 65.01±0.11 & 90.56±0.05 & 36.74±0.84 & 18.16±0.23 & OOM & OOM \\ \hline
        \textbf{HoLe} & \textbf{74.50±0.05} & \underline{72.16±0.07} & \textbf{71.38±0.09} & \textbf{92.45±0.03} & \textbf{91.12±0.01} & \textbf{75.19±0.1} & \textbf{77.13±0.78} & \textbf{61.13} \\
            \bottomrule[0.8pt]
            \end{tabular}
    }
    \label{tab:purity}
\end{table*}

\begin{figure}
    \centering
    \includegraphics[width=0.44\textwidth]{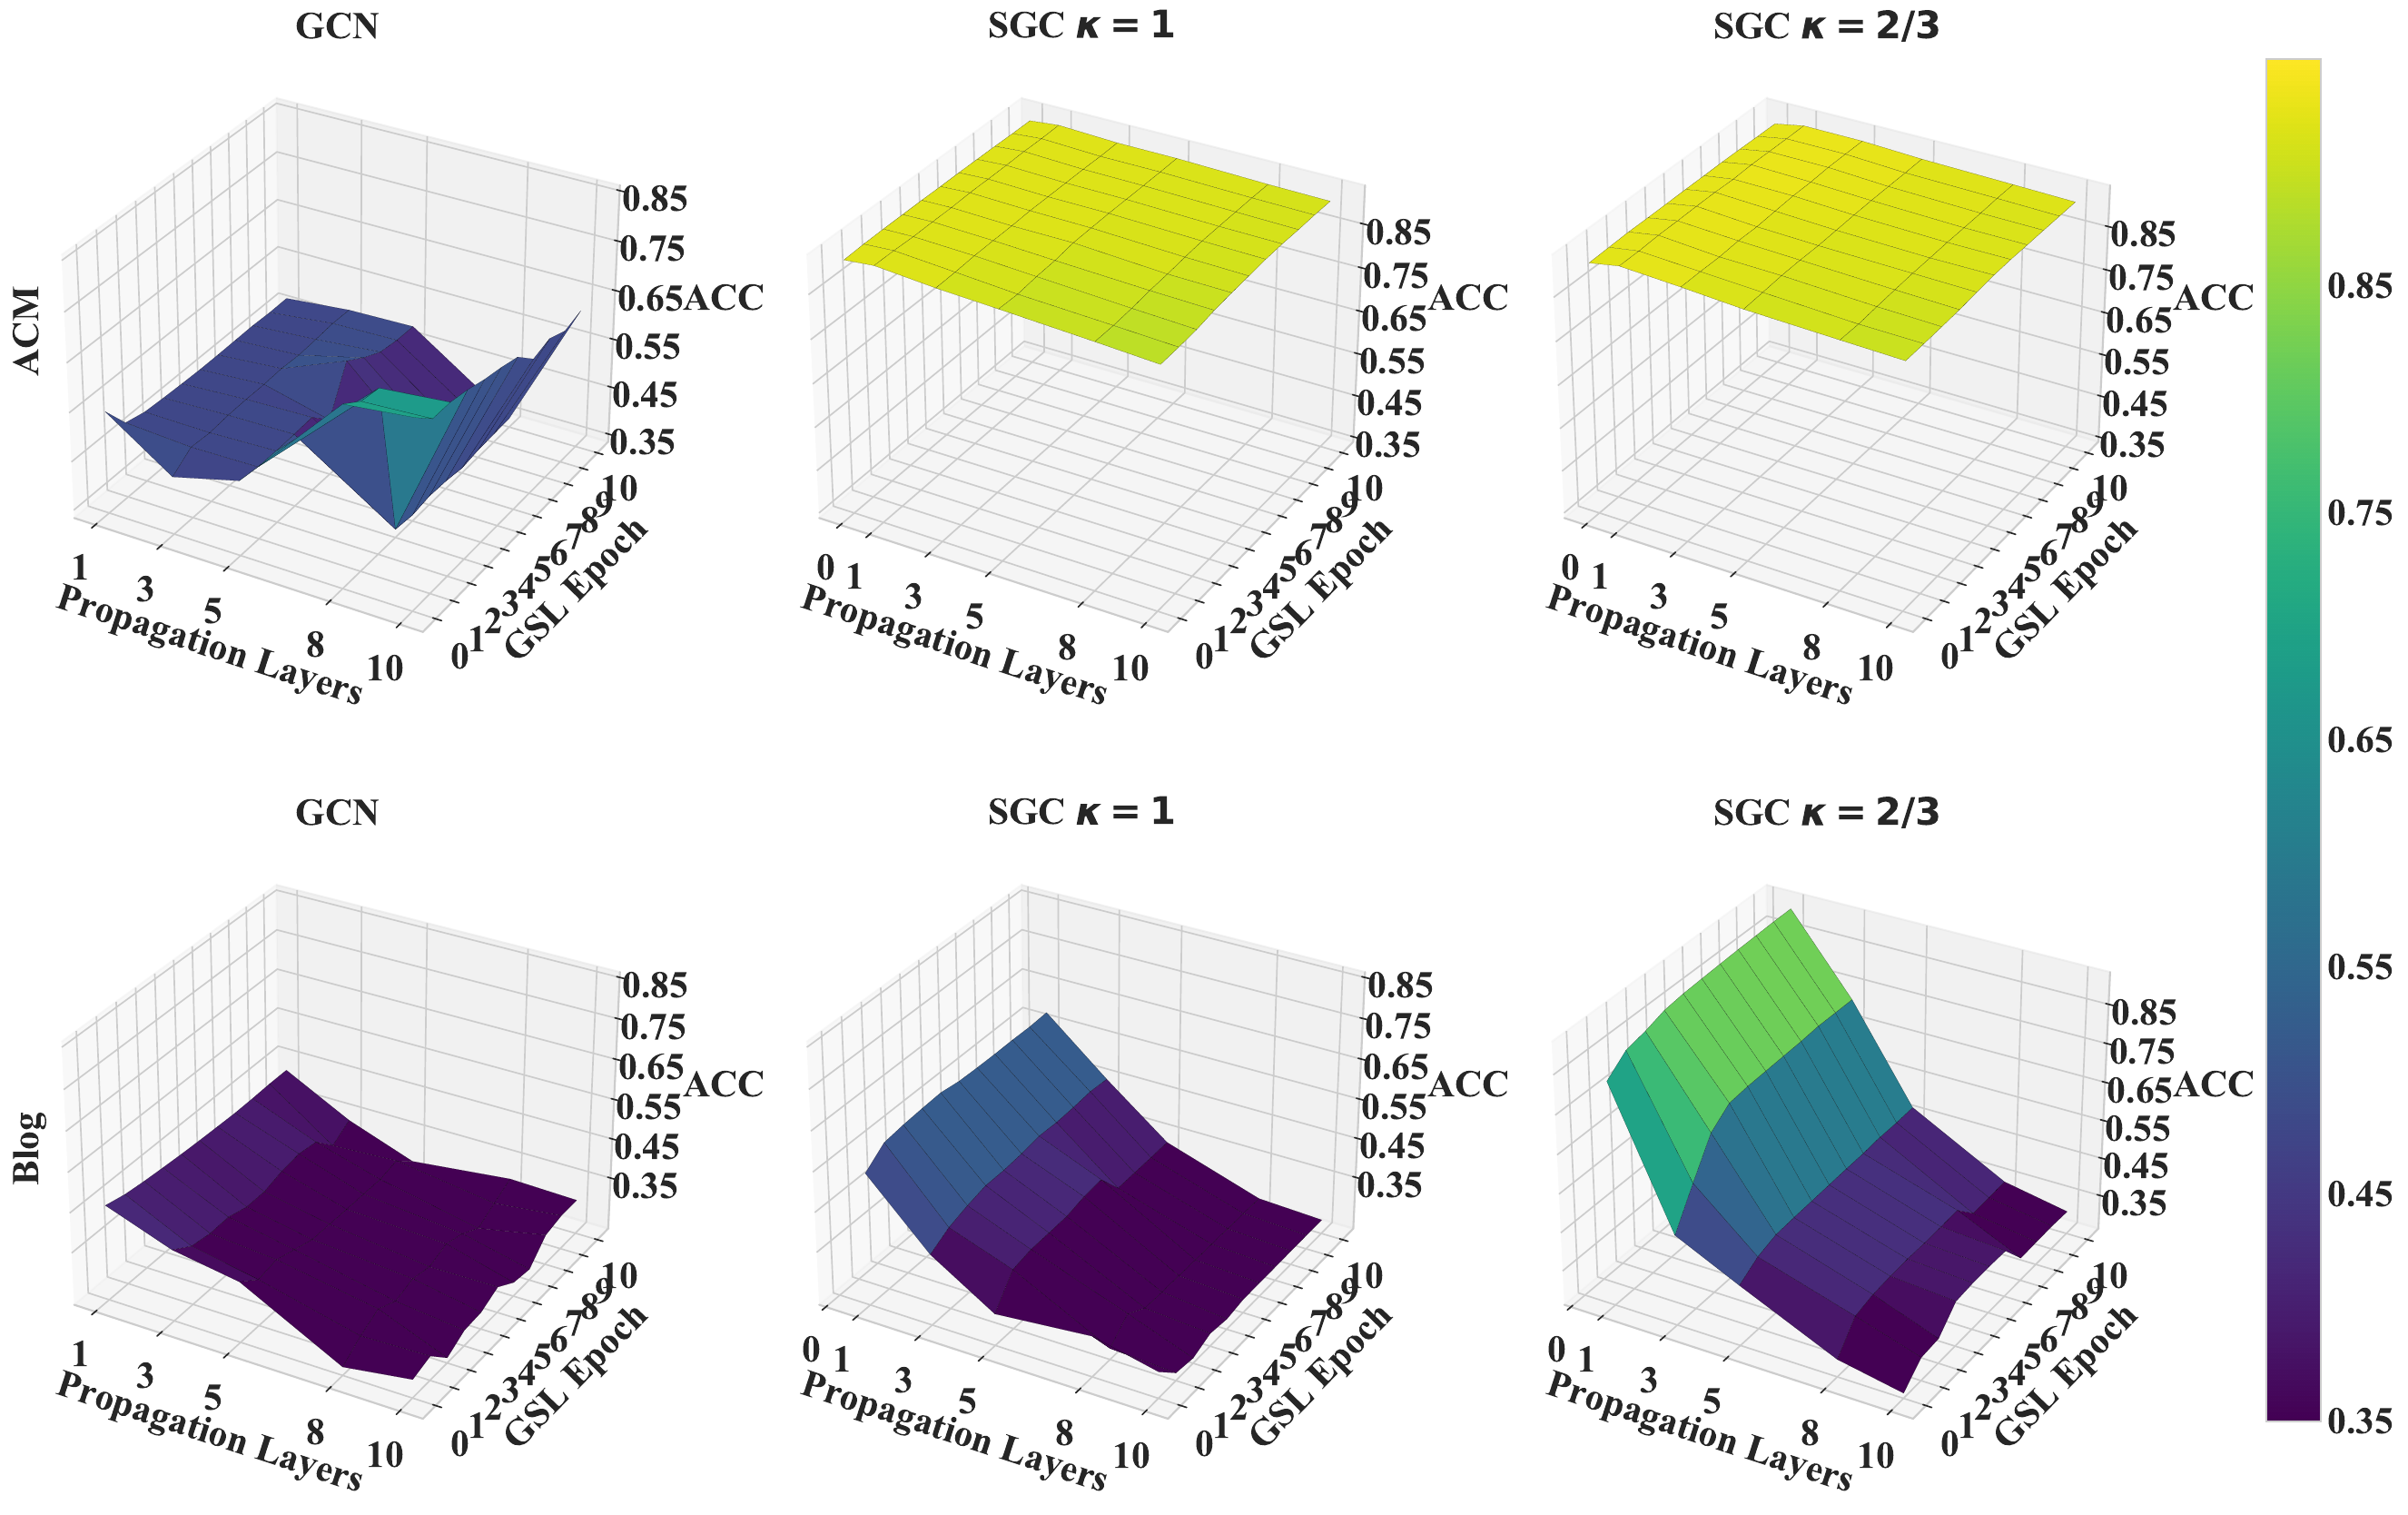}
    \vspace{1em}
    \caption{Performance comparison of \model with different GNN backbones including the vanilla GCN, SGC of $\kappa=1$ and SGC of $\kappa=2/3$. }
    \label{fig:backbones}
\end{figure}

\begin{figure}
    \centering
     \includegraphics[width=0.4\textwidth]{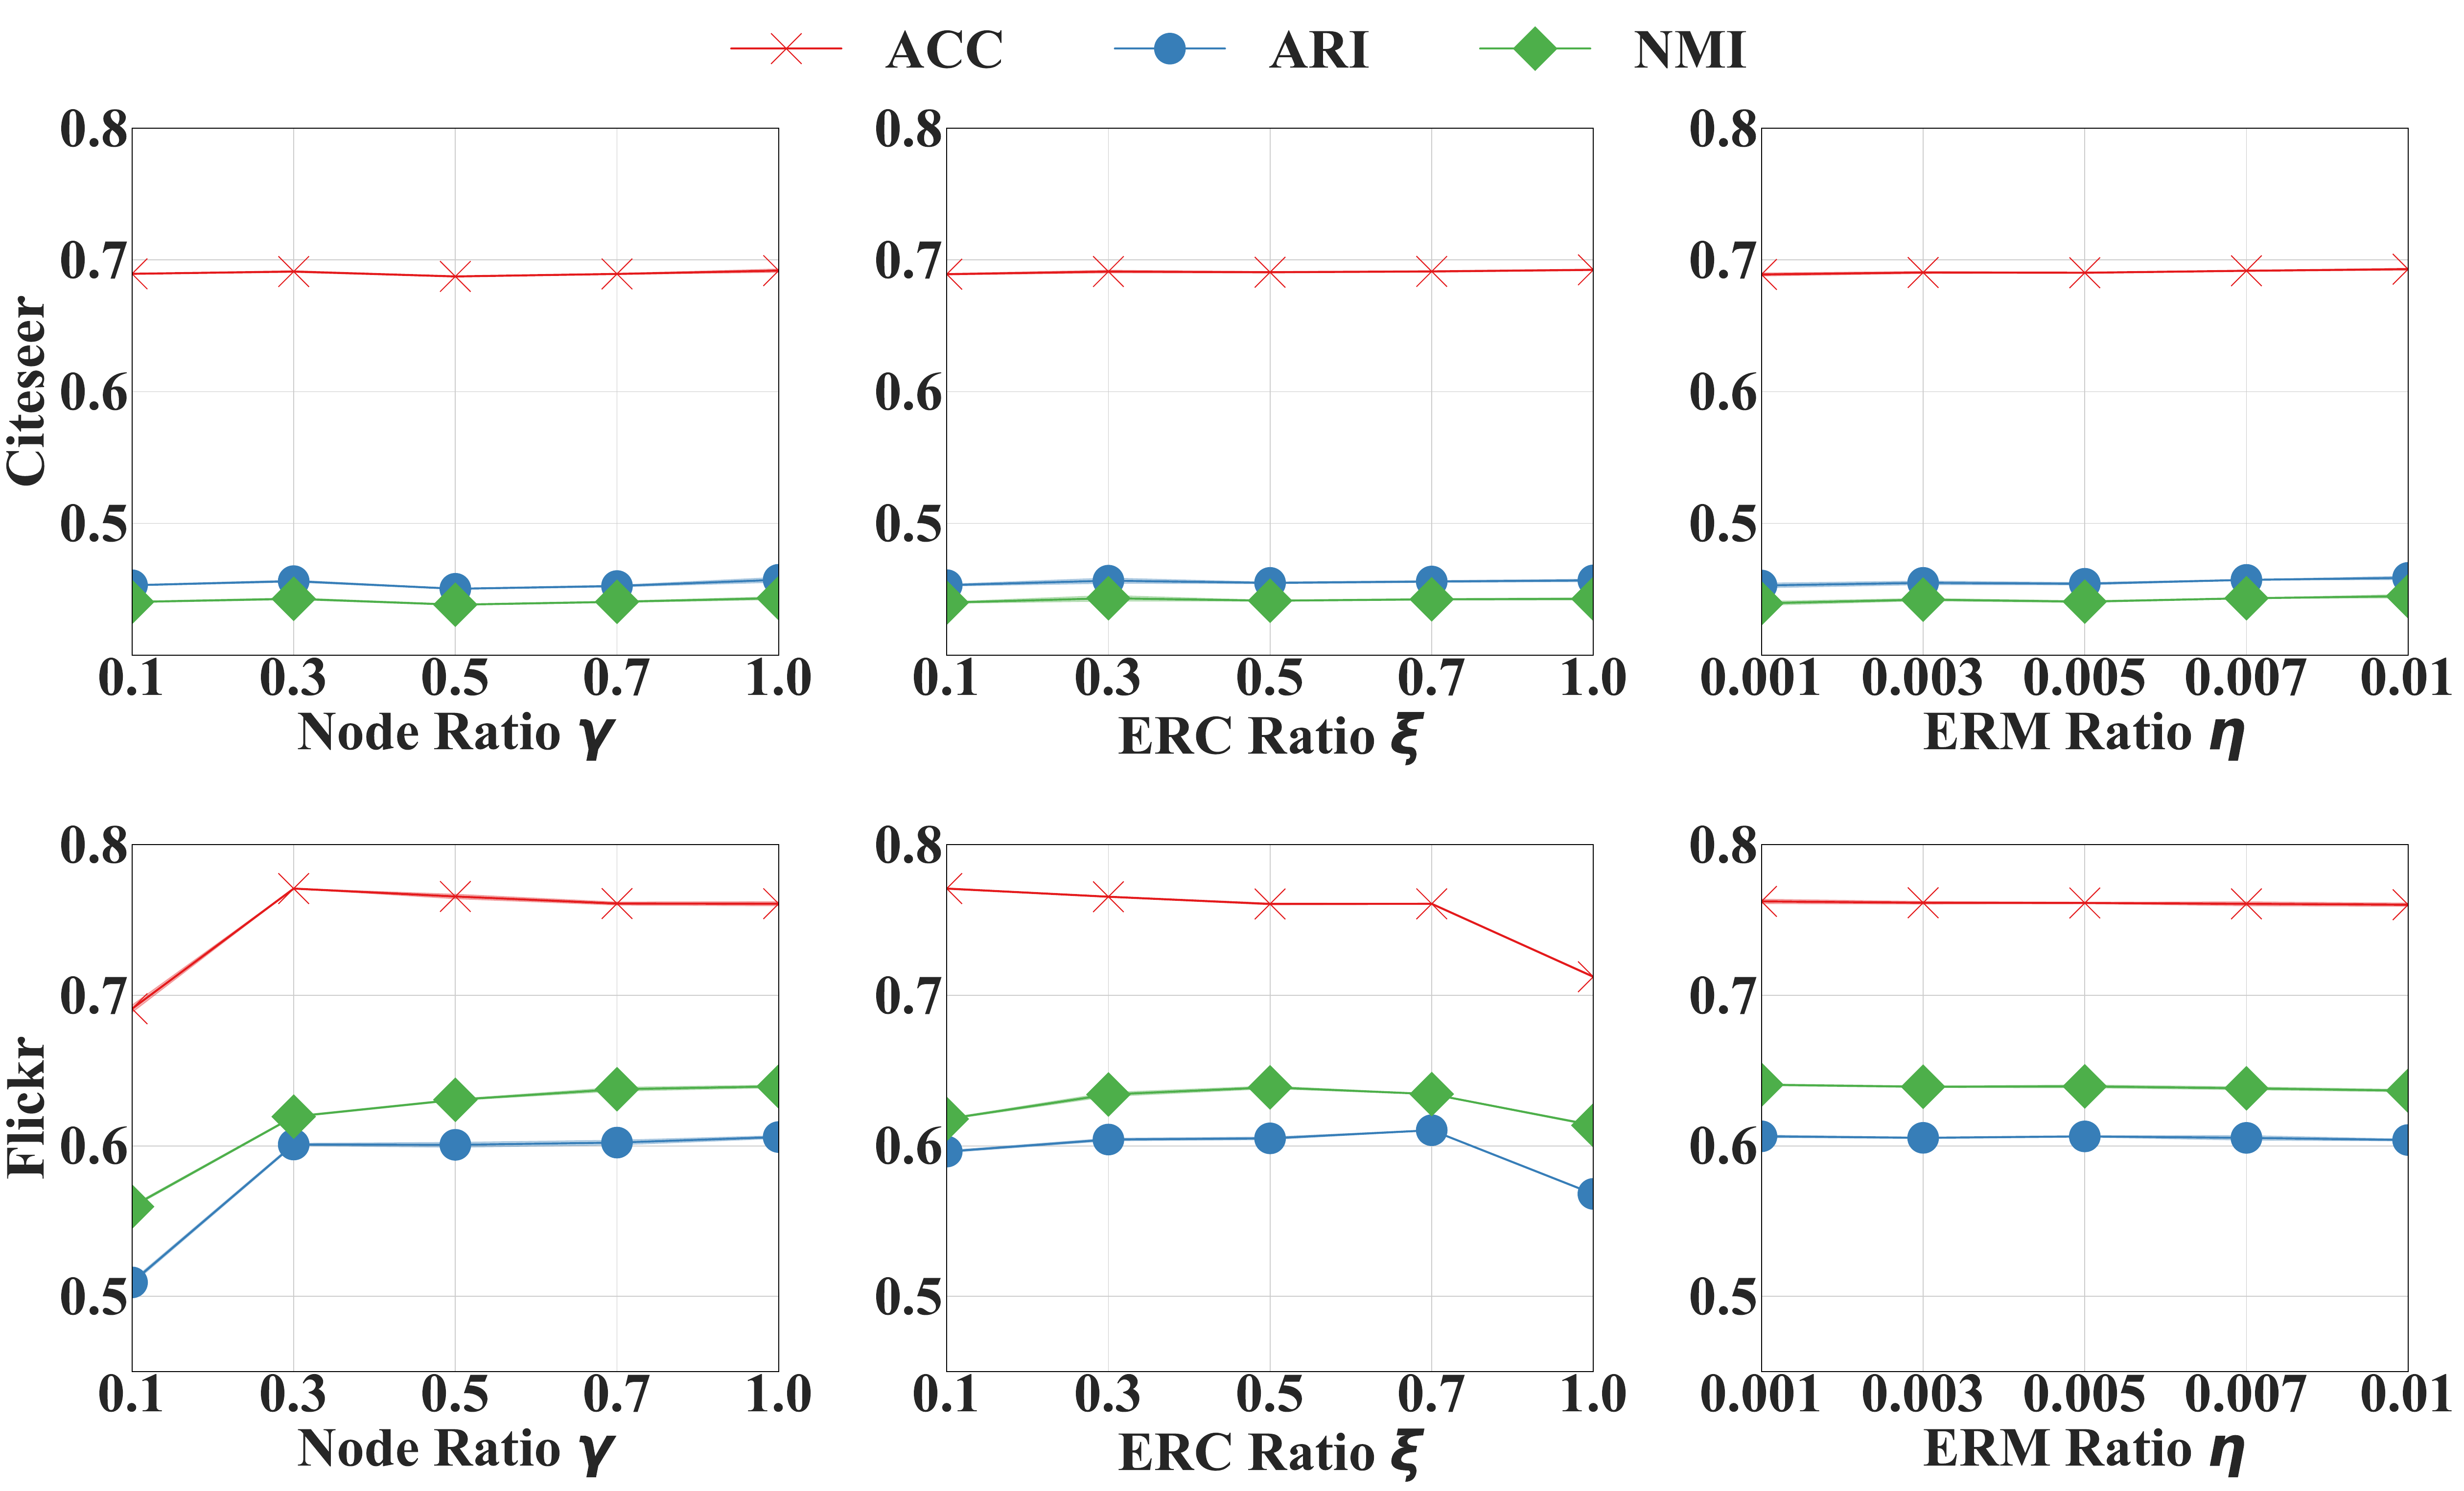}
    \caption{Hyperparameter analysis of high-confidence node extraction ratio $\gamma$, intra-cluster edge recovery (ERC) ratio $\xi$, and inter-cluster edge removal (ERM) ratio $\eta$. }
    \label{fig:param-analysiss}
\end{figure}

\subsection{Choice of GNN backbones for GSL Setting}

As can be seen in Figure \ref{fig:backbones}, on top of the stability of performance improvements as the GSL epoch increases on both citation and social networks, the SGC backbone of $\kappa=2/3$ also shows the advantage of its lower-pass filter~\cite{AGE} over $\kappa=1$.

\subsection{Additional Hyperparameter Analysis.}
Figure \ref{fig:param-analysiss} demonstrates the hyperparameter analysis of two additional datasets not included in the previous section. 
% We use the same experimental setup as Section \ref{sec:hyper-par}. 
It can be seen that the previous conclusions are generally valid.

% It can be seen that the overall fluctuation range is not large on both citation networks, Citeseer and ACM. 
% As regard to the other two social networks, they are more strongly affected by ERC than ERM, but the overall performance generally shows a trend of improvement over the original performance in epoch 0 without structure learning. 
% Because they have relatively lower homophily than Citeseer and ACM, the intra-class edge recovery(ERC) largely optimizes the structure with homophily enhancement.
